# Supplementary material for: Community detection for directed networks revisited using bimodularity
Source: arXiv:2502.04777 source file (2025-07-21)
Supplement: Supplementary file 1 [file BiModularity_SI.pdf]

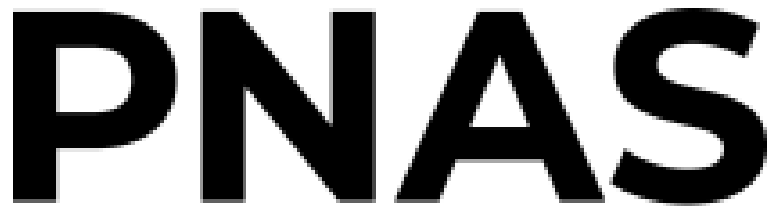

## Supporting Information for

### Community detection for directed networks revisited using bimodularity

Alexandre Cionca, Chun Hei Michael Chan and Dimitri Van De Ville

Dimitri Van De Ville

E-mail: [dimitri.vandeville@epfl.ch](mailto:dimitri.vandeville@epfl.ch)

#### This PDF file includes:

- Figs. S1 to S10
- Legend for Dataset S1
- SI References

#### Other supporting materials for this manuscript include the following:

- Dataset S1

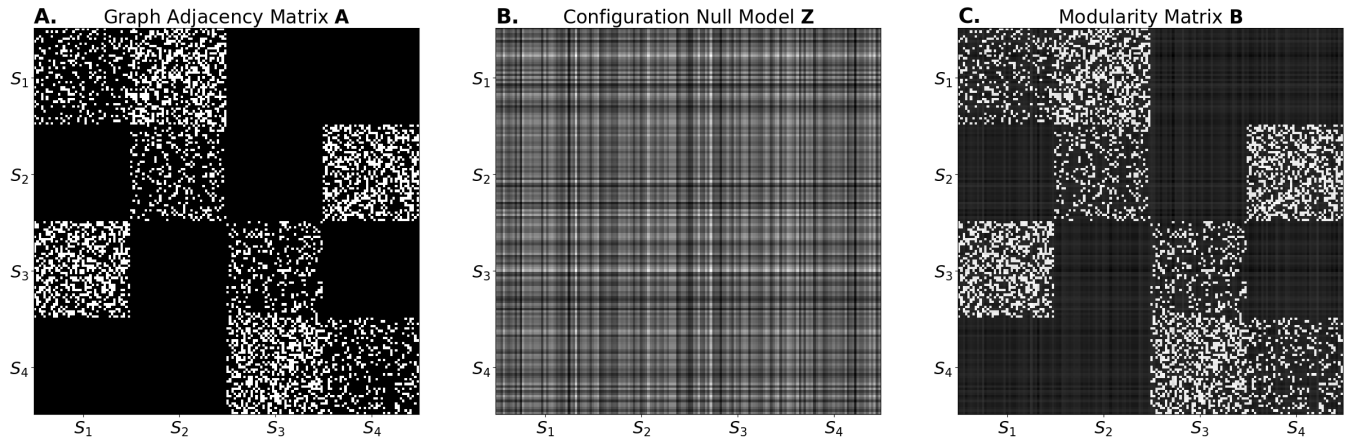

**Fig. S1.** Adjacency, null model and modularity matrices for the canonical block cycle graph. (A) Adjacency matrix  $\mathbf{A}$  of a stochastic block graph of 200 nodes (50 per community) with the structure of A. (B) Configuration null model with the same degree distribution as A. (C) Modularity matrix  $\mathbf{B}$  of A.

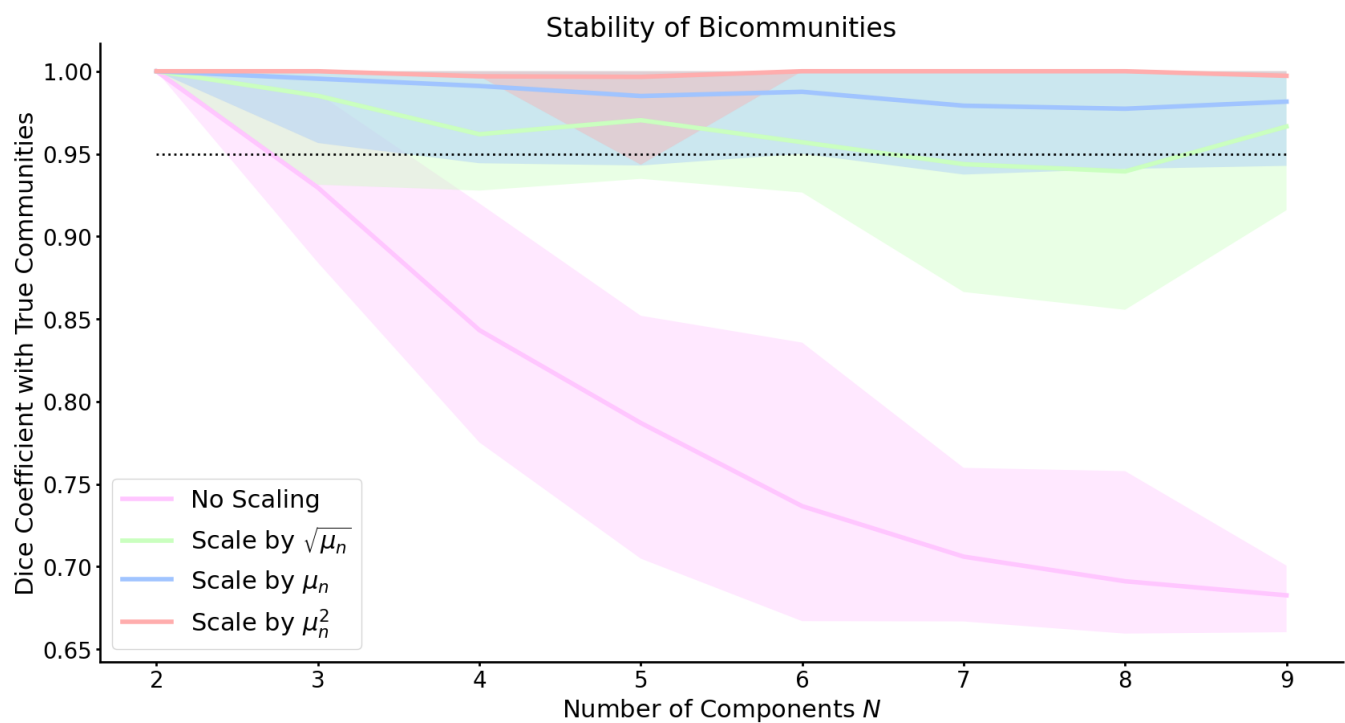

**Fig. S2.** Stability of bicomunity detection in the canonical block cycle graph as measured with the Dice coefficient. The stability is computed as a function of the number of components of the singular value decomposition (SVD – horizontal axis) and for different scaling of the components (colors). The filled area represent the 5 and 95 percentile out of 100 trials. We observe that the scaling of components (even in the case of  $\sqrt{\mu_n}$ ) improves the stability of the detection and that the  $\mu_n$  scaling ensures a similarity higher than 95%.

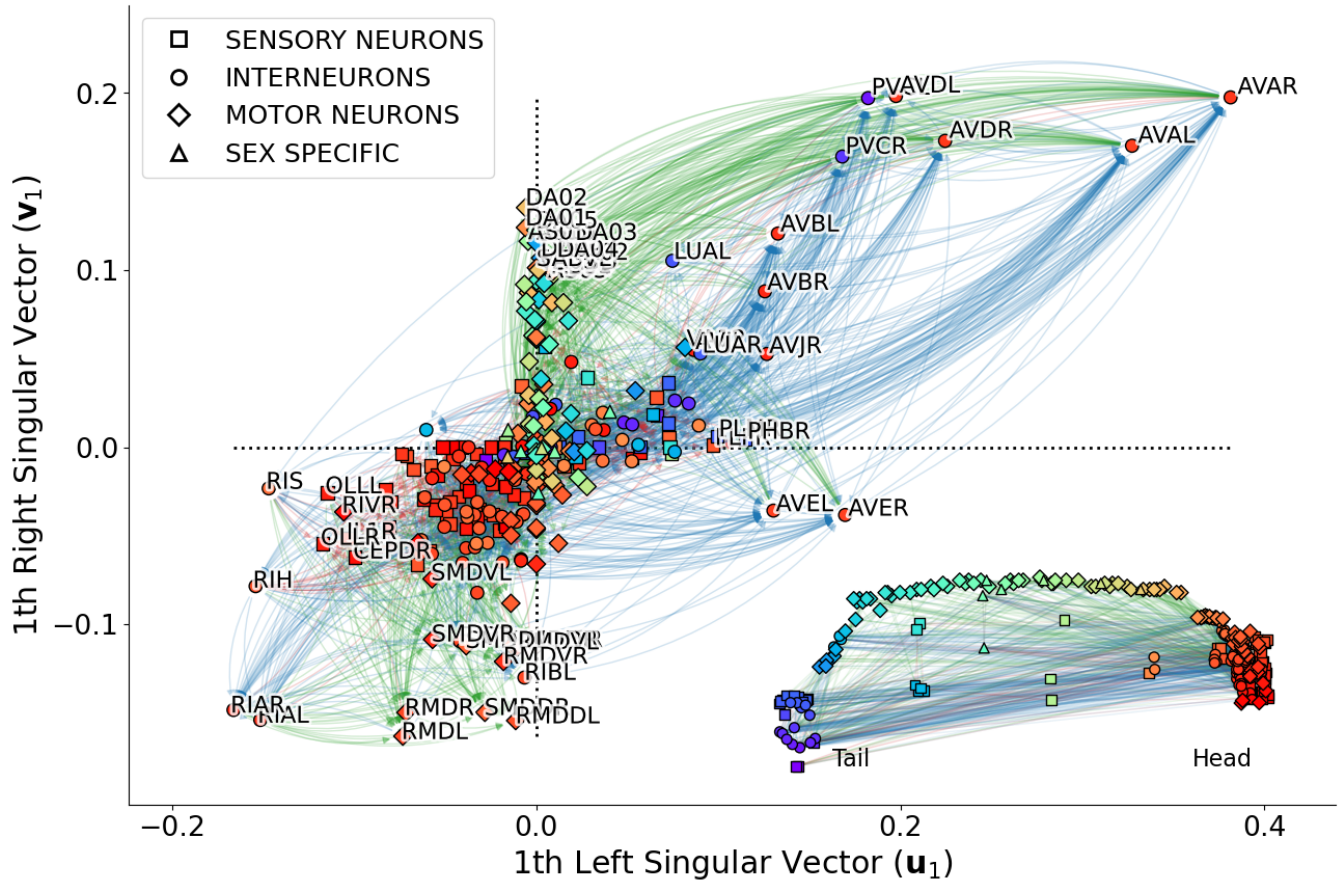

**Fig. S3.** Bimodal embedding of the *C. elegans* wiring network with physical location of neurons. This shows the projection of the graph nodes (neurons) onto the left ( $u_1$ , horizontal axis) and right ( $v_1$ , vertical axis) singular vectors of the bimodal component associated with the largest singular value  $\mu_1$ . Node color indicate the physical location of the neuron in the worm's body from the head (red) to the tail (blue). Shape of nodes indicate the type of the neurons (sensory: square; interneuron: circle; or motor: diamond). Edge colors indicate the type of the target node with red for sensory, blue for inter- and green for motor neurons. Neuron labels are shown for graph nodes that are projected far from the origin (0, 0) of the axes. The legend in the bottom right shows each neuron at their physical location in the worm's body.

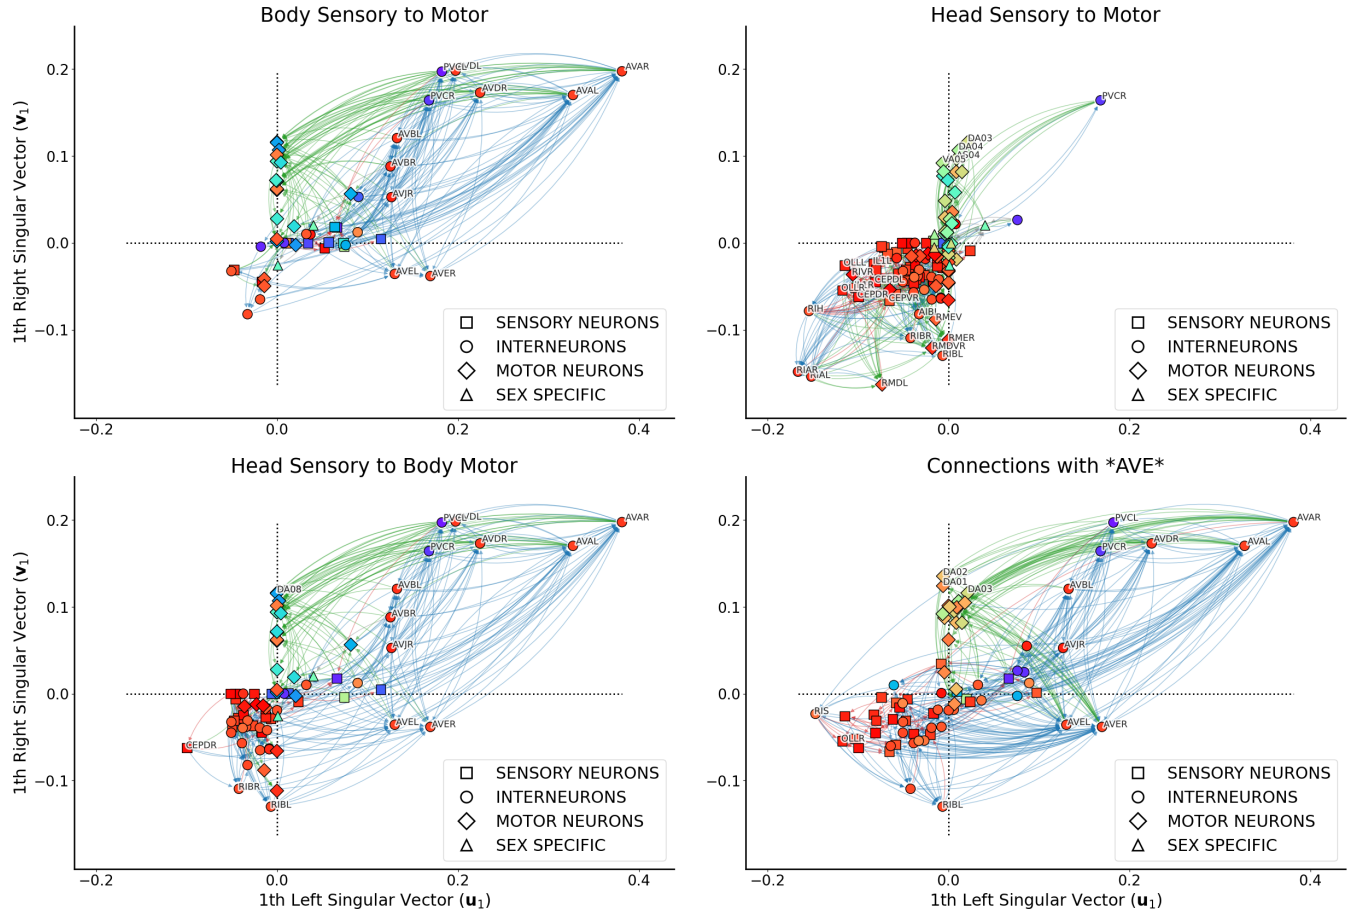

**Fig. S4.** Communication pathways of the *C. elegans* wiring network projected on the first bimodal embedding. Specific pathways are highlighted by discarding all nodes and connections that are not connected to a source (zero in-degree  $k_{in} = 0$ ) or sink (zero out-degree  $k_{out} = 0$ ) node. Sensory to motor communication in the worm's body (top left) is highlighted by considering communication with source nodes on the right half ( $u_1 > 0$ ) and sink nodes on the upper half ( $v_1 > 0$ ). The head sensory to motor pathway (top right) considers communication with source nodes on the left half ( $u_1 < 0$ ) and sink nodes on the lower half ( $v_1 < 0$ ). Finally, head sensory to body motor communication (bottom left) highlights neurons that are linked with left sources and upper sinks. This pathways shares similarities with the bottom right scheme that shows all neurons connected to the AVE interneurons that appear to bridge head sensory inputs and body motor processes. Node color indicate the physical location of the neuron in the worm's body from the head (red) to the tail (blue). Shape of nodes indicate the type of the neurons (sensory: square; interneuron: circle; or motor: diamond). Edge colors indicate the type of the target node with red for sensory, blue for inter- and green for motor neurons. Neuron labels are shown for graph nodes that are projected far from the origin (0, 0) of the axes.



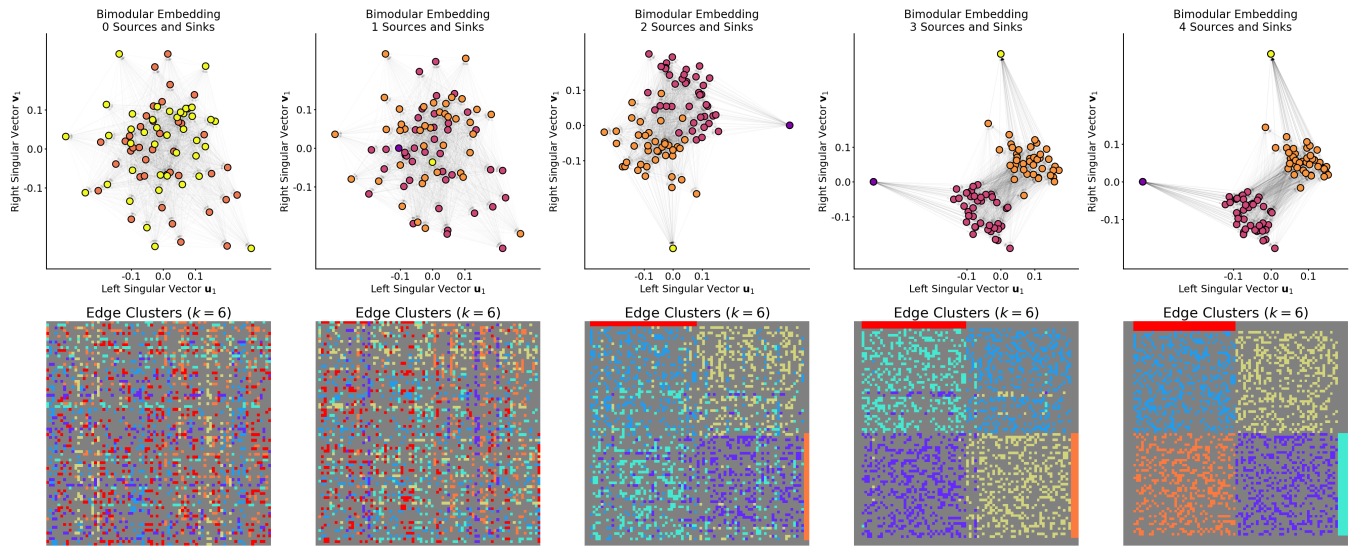

**Fig. S6.** Canonical example of two sets of nodes (red and orange) that are randomly interconnected with the addition of source (purple) and sink (yellow) nodes with high degree imbalance and that connect to either of the node sets. The first row shows the first bimodal embedding of the graph for each number of source and sink node (from 0 to 4). The second row shows the edge clusters as obtained from the bicomunity detection scheme for  $k = 6$  clusters. We observe that 2 added sources/sinks are enough to partially recover the encoded structure and to separate the two sets of nodes. The sources and sinks also are well separated. The two sets are perfectly separated at 3 added nodes and 4 are required to totally recover the 6 clusters of edges.

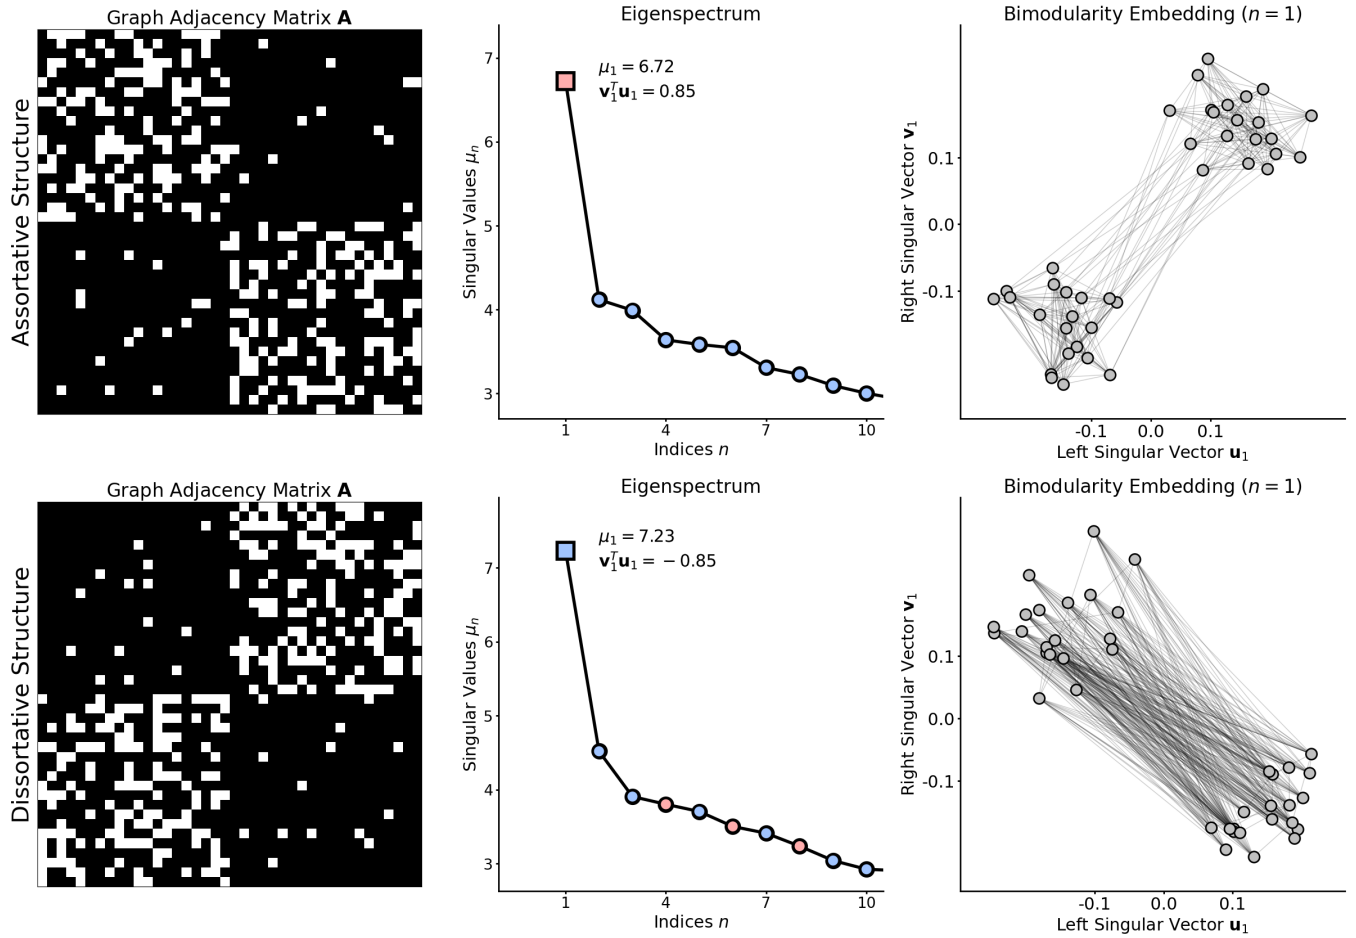

**Fig. S7.** Canonical example of assortative (top) and dissortative (bottom) community structure. While the singular values (middle) have a similar spectrum, we observe a clear difference in the sign convention with  $\mathbf{v}_1^T \mathbf{u}_1 = 0.85$  in the assortative and  $\mathbf{v}_1^T \mathbf{u}_1 = -0.85$  in the dissortative case. The bimodular embeddings (right) show a clear community structure in the assortative graph and a bipartite structure in the dissortative graph. We note that the dissortative embedding separates well the graph nodes in the  $x = -x$  diagonal as opposed to the  $x = x$  diagonal in the assortative condition.



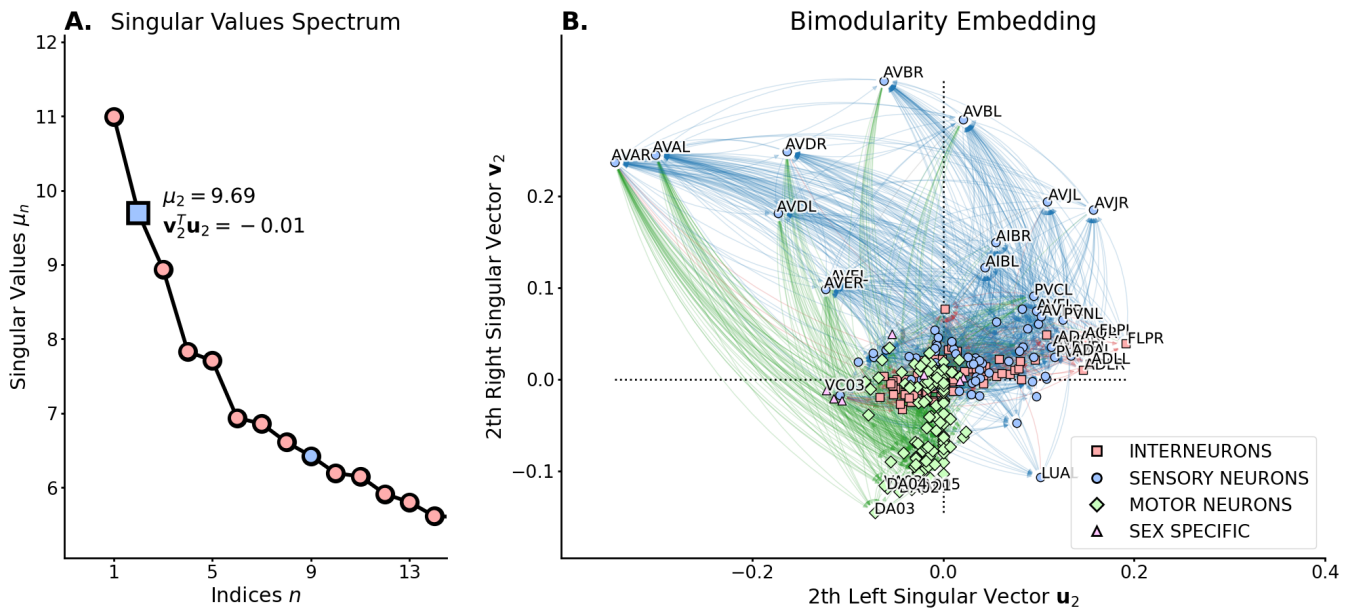

**Fig. S8.** Bimodular embedding of the *C. elegans* wiring network for the 2<sup>nd</sup> component of the Singular value decomposition (SVD). (A) Spectrum of the singular values of the SVD. Colors indicate the sign of the singular value associated to assortative (red,  $\mu > 0$ ) or disassortative (blue,  $\mu < 0$ ) community structures. We observe that while  $\mu_2$  has a high value, this component describes a disassortative structure ( $\mathbf{v}_2^T \mathbf{u}_2 < 0$ ). (B) Projection of the graph nodes (neurons) onto the left ( $\mathbf{u}_2$ , horizontal axis) and right ( $\mathbf{v}_2$ , vertical axis) singular vectors of the bimodular component associated with the largest singular value ( $\mu_2$ ). Colors and shape of nodes indicate the type of the neurons (sensory: red square; interneuron: blue circle; or motor: green diamond). Edge colors indicate the type of the target node with the same color code as for the neuron types. Neuron labels are shown for graph nodes that are projected far from the origin (0, 0) of the axes.

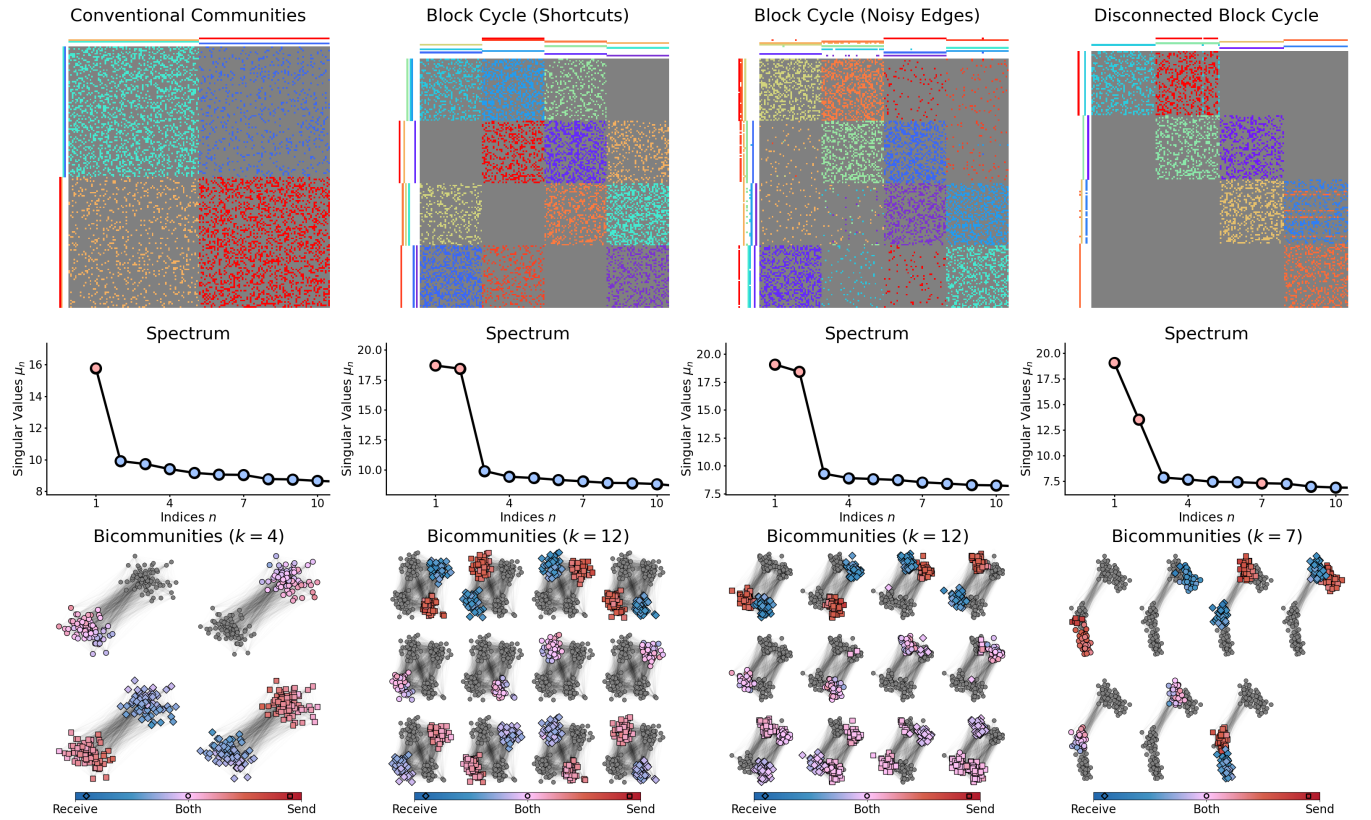

**Fig. S9.** Benchmarking of the bimodularity embedding and bicomunity detection for 4 types of graphs (each column): Conventional community with two sets of nodes that have directed connections within (density 0.6) and between (density 0.24) them; Block cycle graph with bidirectional shortcuts between blocks that are not connected; Block cycle with random edges between nodes; and block cycle with a missing connection between the last and first blocks. The first row shows the adjacency matrix with color corresponding to the edge clusters. In all cases, the encoded structure is recovered and all sets of edges are properly captured in their respective clusters.



## SI Dataset S1 (celegans\_neurons.csv)

This file summarizes the name, type and physical location of neurons used in this article (original data comes from (1–3)).

## References

1. LR Varshney, BL Chen, E Paniagua, DH Hall, DB Chklovskii, Structural Properties of the Caenorhabditis elegans Neuronal Network. *PLOS Comput. Biol.* **7**, e1001066 (2011) Publisher: Public Library of Science.
2. SJ Cook, et al., Whole-animal connectomes of both Caenorhabditis elegans sexes. *Nature* **571**, 63–71 (2019) Publisher: Nature Publishing Group.
3. CA Brittin, SJ Cook, DH Hall, SW Emmons, N Cohen, Volumetric reconstruction of main Caenorhabditis elegans neuropil at two different time points (2018) Pages: 485771 Section: New Results.
